# Supplementary material for: DeepProcess: Supporting business process execution using a MANN-based recommender system
Source: arXiv:1802.00938 source file (2021-11-23)
Supplement: Supplementary file 1 [file appendix.tex]

\section{Appendix: Predictive Process Monitoring with MANN}

To further establish the efficacy of our proposed architecture we evaluate it on the task of suffix prediction(next best course of action, given a partially executed process instance). Here baseline is the state-of-the-art multi-layer LSTMs model
introduced in \cite{tax2017predictive}. We pick the best results reported in \cite{tax2017predictive} for the task of suffix prediction and compare
them with results obtained using our model. 

\textbf{Datasets for benchmarking:} 

There are two datasets previously studied and pre-processed in \cite{tax2017predictive}:
\begin{itemize}
    \item  \textbf{Helpdesk:} This log contains events from a ticketing management process of the help desk of an Italian software company. The process consists of 9 activities, and all cases start with the insertion of a new ticket into the ticketing management system. Each case ends when the issue is resolved and the ticket is closed. This log contains around 3,804 cases and 13,710 events, which results in about 14K training and 4K testing samples.
    \item \textbf{BPI'12:} This event log originates from the Business Process Intelligence Challenge (BPI’12) and contains data from the application procedure for financial products at a large financial institution. The training and testing size for this dataset are about 40K and 10K samples, respectively. BPI’12 (no duplicate): Besides BPI’12, the authors of \cite{tax2017predictive} also create a simpler version of Business Process Intelligence Challenge data. This version removes repeated occurrences of the same event, keeping only the first occurrence, which is suitable for suffix prediction task. There are about 19K training 8.4K testing samples in this dataset.
\end{itemize}

\begin{table}
\begin{centering}
\begin{tabular}{|l|c|c|}
\hline 
Model & Helpdesk & BPI'12 W ({*})\tabularnewline
\hline 
Tax \emph{et al.} \cite{tax2017predictive} & 0.767 & 0.394\tabularnewline
MANN & \textbf{0.772} & \textbf{0.417}\tabularnewline
\hline 
\end{tabular}
\par\end{centering}
\caption{Suffix Prediction Task: Damerau-Levenshtein Similarity (higher is
better). ({*}) no duplicate.\label{tab:Suffix-Prediction-Task}}

\end{table}

To benchmark our technique with the existing results, we use the same preprocessing as in [21] to extract a feature vector for each event in a business
process. The training and testing data are also prepared in the same way as in
\cite{tax2017predictive} for fair comparison. We use the Damerau-Levenshtein Similarity, which is
approximately equal to 1-normalized edit distance. To be fair, we also use the same
prediction algorithm proposed in their paper to perform suffix prediction for
these datasets. We observe that the MANN performs better than the highly-tuned architecture in \cite{tax2017predictive}.

%In these tasks, the metrics used are Accuracy for the next activity
%prediction and Mean Absolute Error (MAE) for time-to-event estimation.
%We evaluate on the two preprocessed-feature datasets: Helpdesk and
%BPI'12 in the same manner as \cite{tax2017predictive}, that is in
%training, we train our MANN with two loss functions (Accuracy and
%MAE) jointly and in testing, our MANN predicts the next activity and
%its time-to-event at the same time. 

%The results are reported in Table~\ref{tab:DCw-MANN-hyper-parameters}.

%We use same datasets (Helpdesk, BPI’12 no duplicate), to make it comparable with [21], 
